# Supplementary material for: Source Identification in Abstractive Summarization
Source: arXiv:2402.04677 source file (2024-02-07)
Supplement: Supplementary file 1 [file noappendix.tex]

\begin{table*}[t]
    \centering
    \footnotesize
    \begin{tabular}{p{\linewidth}}
        \toprule
        \textbf{Generated summary:} A group of Silicon Valley heavyweights has pledged \$1bn (£700m) to fund research into artificial intelligence.\\\midrule
        \textbf{Input document:}
        \hl{ggreen}{(S1) The venture's backers include Tesla Motors and SpaceX CEO Elon Musk, Paypal co-founder Peter Thiel,} \hl{ggreen}{Indian tech giant Infosys and Amazon Web Services.}\ppltag{1}
        (S2) Open AI says it expects its research - free from financial obligations - to focus on a "positive human impact".\rougetag{2}\ppltag{3}
        (S3) Scientists have warned that advances in AI could ultimately threaten humanity.\bertscoretag{1}
        (S4) Mr Musk recently told students at the Massachusetts Institute of Technology (MIT) that AI was humanity's "biggest existential threat".\attentiontag{2}
        (S5) Last year, British theoretical physicist Stephen Hawking told the BBC AI could potentially "re-design itself at an ever increasing rate", superseding humans by outpacing biological evolution.
        (S6) However, other experts have argued that the risk of AI posing any threat to humans remains remote..\rougetag{3}\bertscoretag{3}\attentiontag{3}
        \hl{ggreen}{(S7) A statement on OpenAI's website said the venture aims "to advance digital intelligence in the way that is most likely to} \hl{ggreen}{benefit humanity as a whole, unconstrained by a need to generate financial return".}
        (S8) "It's hard to fathom how much human-level AI could benefit society, and it's equally hard to imagine how much it could damage society if built or used incorrectly."
        (S9) The statement said AI "should be an extension of individual human wills and, in the spirit of liberty, as broadly and evenly distributed as is possible safely".\attentiontag{1}
        \hl{ggreen}{(S10) It said only a tiny fraction of the \$1bn pledged would be spent in the next few years.}\rougetag{1}\bertscoretag{2}\ppltag{2} \\
        \bottomrule
    \end{tabular}
    \caption{Example 2 (XSum)}
    \label{tab:example_b}
\end{table*}

\begin{table*}[t]
    \centering
    \footnotesize
    \begin{tabular}{p{\linewidth}}
        \toprule
        \textbf{Generated summary:} A campaign group has called on the UK government to scrap employment tribunal fees.\\\midrule
        \textbf{Input document:} 
\hl{ggreen}{(S1) The Citizens Advice Bureau in Scotland said fees had "altered the balance of power" between workers} \hl{ggreen}{and employers since they were introduced in 2013.}\ppltag{1}
(S2) People face fees of up to Â£1,200 for their claims to be heard by a tribunal.
(S3) The UK Ministry of Justice said fee waivers were available for those who could not afford to pay.\bertscoretag{3}
(S4) The Citizens Advice Bureau's Price of Justice report, published jointly with Strathclyde University, revealed the number of tribunal cases lodged during the first quarter of last year fell by 81\% compared with the same period 12 months previously.
\hl{ggreen}{(S5) Citizens Advice Scotland (CAS) spokeswoman Lauren Wood said: "A few weeks} \hl{ggreen}{ago we published CAB evidence showing that the number of Scots being exploited at work was increasing.}
(S6) "Today we publish a new report which shows how such workers are being prevented from getting the justice and compensation they are entitled to.
(S7) "It's two years since the government introduced a fee for employment tribunals.\rougetag{1}\bertscoretag{1}\ppltag{3}
(S8) "The evidence shows that people have been deterred from taking their grievances to tribunal because they simply can't afford to pay the fee."
(S9) She added: "One of the most worrying aspects of this current situation is that it has altered the balance of power at work, with rogue employers now feeling they can exploit or mistreat their employees without risk of being called to account.\attentiontag{2}
\hl{ggreen}{(S10) "In highlighting this issue today we call on the government - and all political parties - to think again about the price of} \hl{ggreen}{justice, and to get rid of these fees.}\rougetag{3}\bertscoretag{2}\attentiontag{3}\ppltag{2}
(S11) "Justice should be available to everyone, not just the wealthy."
(S12) A Ministry of Justice spokesman said: "We want people to resolve these issues using quicker and simpler alternatives such as arbitration and mediation and only go to court as a last resort.\attentiontag{1}
(S13) "We have made sure fee waivers are available for those who can't afford to pay, as well as diverting people away from potentially acrimonious hearings, where possible, through a new early conciliation scheme which has already been used by over 60,000 people in its first nine months.
(S14) "The government has committed to reviewing employment tribunal fees but believes this is better determined by the new administration following the election."\rougetag{2}\\\bottomrule
    \end{tabular}
    \caption{Example 3 (XSum)}
    \label{tab:example_c}
\end{table*}
